# Supplementary material for: Silicon liquid structure and crystal nucleation from ab-initio deep Metadynamics
Source: arXiv:1809.11088 ancillary file (2019-01-09)
Supplement: Supplementary file 1 [file supplementary.pdf]

Supplemental information to:

# Silicon liquid structure and crystal nucleation from *ab-initio* deep Metadynamics

Luigi Bonati and Michele Parrinello

## CONTENTS


I. Molecular Dynamics setup 1

II. DFT calculations 2

III. DeePMD training and testing 2

IV. Local Structure Factor 6

A. Implementation 6

B. Fingerprint 7

References 9


## I. MOLECULAR DYNAMICS SETUP

MD simulations are performed using LAMMPS [1]. A Velocity Verlet integrator is employed with a timestep of 1 fs. Isothermal and isobaric simulations are performed around the melting point at ambient pressure using the Stochastic Velocity Rescaling Thermostat [2] and the Parrinello-Rahman barostat [3] integrated with the one of Martyna *et al.* [4]. The relaxation times for the thermostat and the barostat are set at 0.1 ps and 10 ps, respectively. The simulations for the training set use the Stillinger-Weber empirical potential for Si [5]. The number of atoms is 216, corresponding to a 3x3x3 supercell. For the simulations with the DeePMD potential system sizes of 216, 1728 and 4096 are used.

The calculation of the collective variables and of the Metadynamics bias are done with PLUMED 2 [6], patched with LAMMPS. PLUMED is used also for post-processing the data in order to recover the free energy surface.

## II. DFT CALCULATIONS

DFT [7] electronic structure calculations are performed using the Quickstep [8] module of the CP2K program[9].

The SCAN exchange and correlation functional is used via LIBXC 3.0.1 library [10].

Goedecker-Teter-Hutter (GTH) [11, 12] pseudopotentials are used to represent core electrons (optimized for PBE). A family of Gaussian basis sets (MOLOPT) is used [13], in the version optimized for condensed matter systems with the GTH-PPS.

The single point energy and forces calculations for the training set use a energy cutoff of 400 Ry. The threshold for the energy convergence is set to $10^{-11}$ and the one related to SCF cycles is set to $10^{-6}$.

To deal with metals configurations we use a Fermi Dirac smearing of the occupation number around Fermi energy (0.025 eV), together with a mixing of the electronic density in k-space, to avoid possible effects of charge sloshing (Kerker Mixing).

A 2x2x2 k-points grid (corresponding to a grid spacing of 0.03 $\AA^{-1}$) is used. While for the cubic diamond structure also a gamma point calculation with a 3x3x3 supercell is enough, in order to get a correct description of the $\beta$-tin energy is crucial to use a finer grid.

Additional AIMD simulations have been performed within the Born-Oppenheimer approximation in order to create a benchmark for the DeePMD potential. NVT simulations of the liquid (at 1800K) and the solid (at 1700K) are performed. The equations of motion are integrated with a timestep of 0.5 fs, and the temperature is maintained at the desired temperature with the Stochastic Velocity Rescaling Thermostat [2], employing a coupling constant of 50 ps.

## III. DEEPMD TRAINING AND TESTING

The DeePMD-kit [14] package is used for the training of the neural network potential and to interface the NN potential to LAMMPS.

A neural network with 5 hidden layers is used, with a number of neurons per layer equal to [240, 120, 60, 30, 10].

In order to build the descriptors which are invariant under the relevant symmetries, a local reference frame is built for every atom, based on the two closest neighbors atoms.

The network is trained for 800 epochs with the ADAM optimizer, with an exponentially decaying learning rate going from 1e-3 to 3.5e-8. The prefactors of the energy and the force terms in the loss functions change during the optimization process from 0.02 to 8 and from 1000 to 1 respectively.

The total number of training configurations is 30k, composed by a dataset of 24K from the MetaD simulation and a dataset of 6k snapshots extracted from equilibrium AIMD simulations of the two phases.

The energy converges smoothly as a function of the number of configurations included into the training set, as it is reported in fig. SI-1.

In fig. SI-2 the RMSE as a function of the energy is reported, showing how equilibrium configurations are better reproduced with respect to intermediate ones.

We have also computed the radial distribution function of both the solid and the liquid (fig. SI-3). The latter is an important benchmark, since an accurate description of the liquid requires a discrimination of the metallic and covalent bonding. We compared it with the results of AIMD simulations, and the result is remarkable.

Regarding the generality of the training set, this can be assessed by training two or more NN potentials initialized with different parameters, and checking their prediction on a dynamics driven by one on them [15]. If their predictions differ too much, these configurations need to be included into the training set. We checked these errors on a short WTMetaD simulation in which the system visited both states, and the errors are comparable to the ones obtained with the testing set, meaning that our initial set is already robust and general for the purpose of this work.

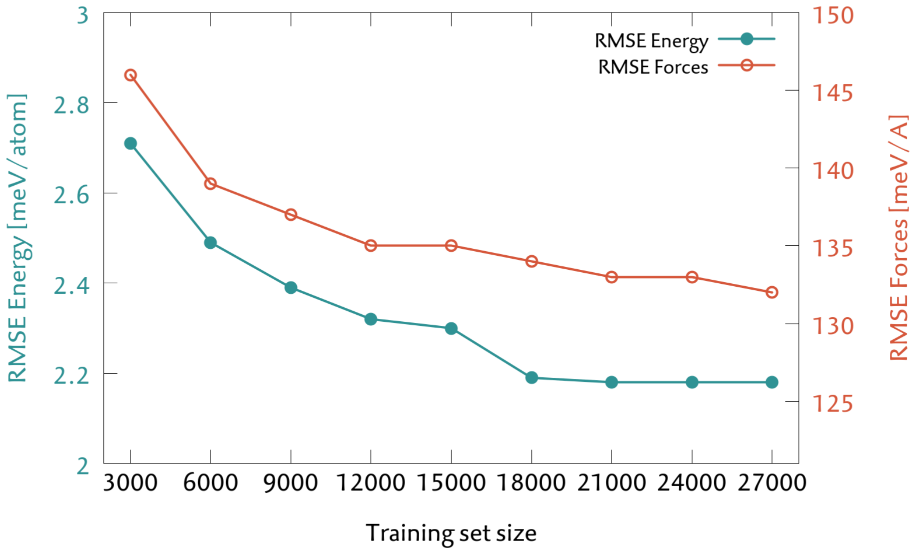


FIG. SI-1. Root Mean Square Error versus data size of the training set. The errors are computed on a training set of 3k configurations which contains both data from the MetaD simulation and from equilibrated AIMD simulations.

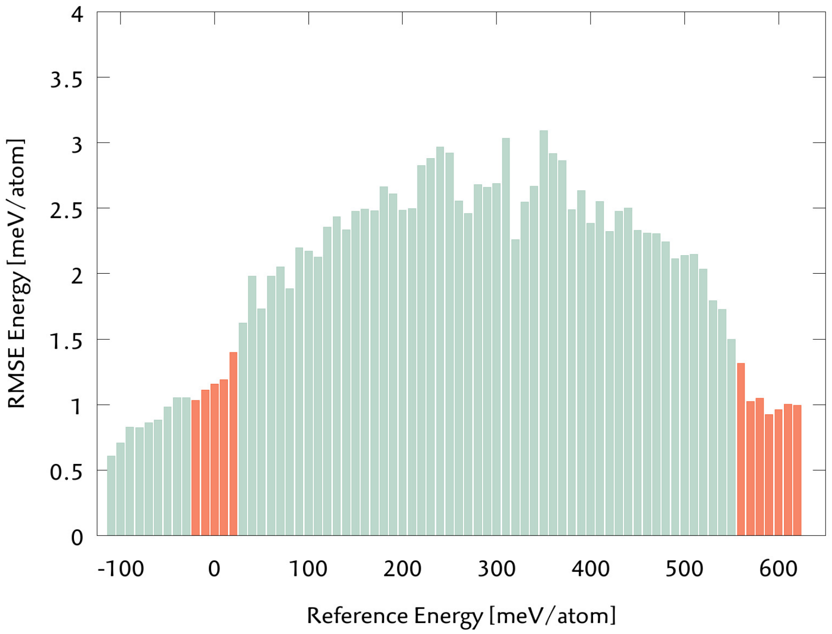


FIG. SI-2. Root Mean Square Error as a function of the energy for the DeePMD potential trained for silicon. The testing set is composed of data from the WTMetaD simulation together with data from AIMD simulation on the solid and the liquid (whose energy range is marked in red). The energies on the x-axis are shifted by the mean value of the solid from AIMD ad 1700K.

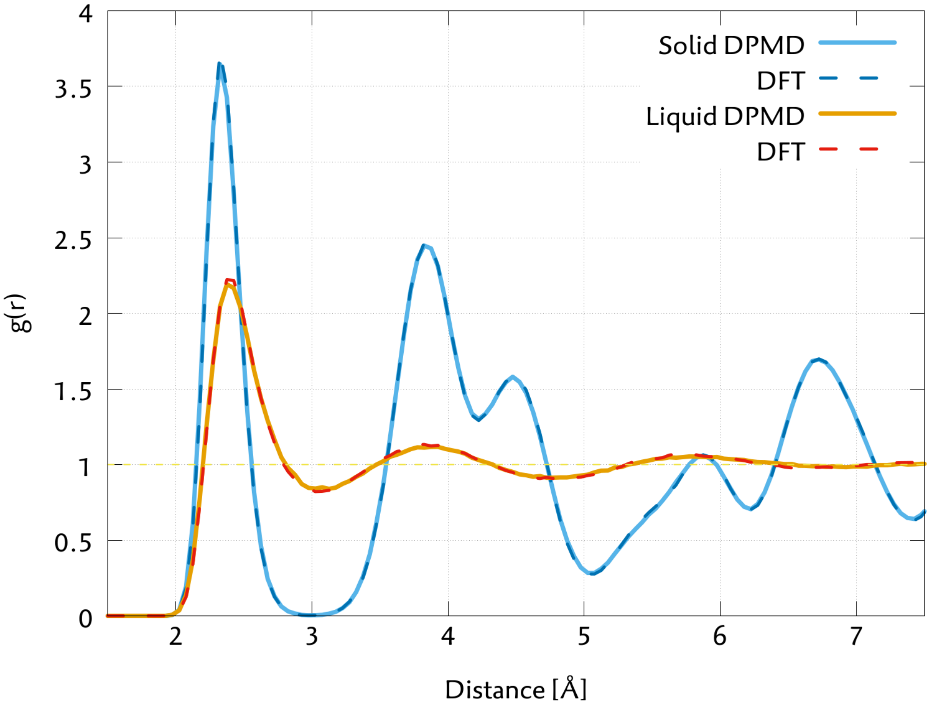


FIG. SI-3. Radial Distribution Function of the two phases, computed with the DeePMD potential. Reference data are from AIMD simulations.

## IV. LOCAL STRUCTURE FACTOR

### A. Implementation

The local structure factor is programmed in a private version of PLUMED 2, and it is defined as:

$$S_i(q) = 1 + \sum_{j \neq i}^{N_n} \frac{\sin(\pi r_{ij}/r_c)}{\pi r_{ij}/r_c} \frac{\sin(q\, r_{ij})}{q\, r_{ij}} \tag{1}$$

The first term is a window (or damping) function needed to alleviate the termination effects caused by the finite cutoff [16, 17]. The reason is that if the pair correlation function is not flat at the cut-off distance we have to damp it, in order to make the contributions vanishing for $r \sim r_c$.

We note that the average of $S_i(q)$ over all the atoms gives the structure factor as given by the Debye equation (approximated with the same cutoff).

It is implemented in the MULTICOLVAR framework, meaning that an array of per-atom values is created. Then one can compute functions of these quantities like MEAN, MIN, MAX, and also study their distributions.

In this work the number of atoms whose $S_i(q)$ is greater than a threshold value is used as a CV. This is computed as:

$$n = \sum_{k=1}^{N} 1 - \sigma(\bar{S} - S_i) \tag{2}$$

where $\sigma(x)$ is a differentiable switching function that goes to 1 for $x < 0$ and to 0 otherwise.

We report an example of a PLUMED input file for the calculation of the $S_i(q)$ used in this work. The first peak of solid Si, located at 1.98 Å, is chosen. Then the local structure factor is computed by counting the contribution of the neighbors up to a cut-off distance of 8 Å. In addition, two scalar quantities are computed: the MEAN value across all the particles and the number of solid-like atoms, by filtering how many atoms have a structure factor above a target of 1.2 (MORE_THAN).

```
LOCAL_STRUCTURE_FACTOR ...
 LABEL=lsq
 SPECIES=1-1728
 CUTOFF=8.0
 ACTIVE_Q=1.98
 MEAN
 MORE_THAN={RATIONAL R_0=1.25 NN=12 MM=24}
... LOCAL_STRUCTURE_FACTOR
```

### B. Fingerprint

The structure factor can be used also as an atomic fingerprint, to distinguish between solid and liquid particles. Provided that the cutoff radius contains a few neighbors shells, this parameter is able to detect the presence of an ordered environment.

In figure SI-4 a liquid-solid interface is presented, where the atoms are coloured according to their $S_i(q_1)$ values above a threshold of 1.25 (see fig. 1 of the letter). This is compared with the extended version of Common Neighbour Analysis implemented in the visualization software OVITO [18]. The agreement is remarkable, and it is a pratical example of how the local structure factor can be used as a continuous and differentiable crystallinity order parameter.

If one peak alone is not able to distinguish the solid from the liquid or different structures, we can sum the information of two or more peaks to build the local order parameter. Furthermore, the generalization to multi-component systems is straightforward, since we just have to weight the contributions by the atomic scattering factors, thus recovering the diffraction intensity in the spirit of [19].

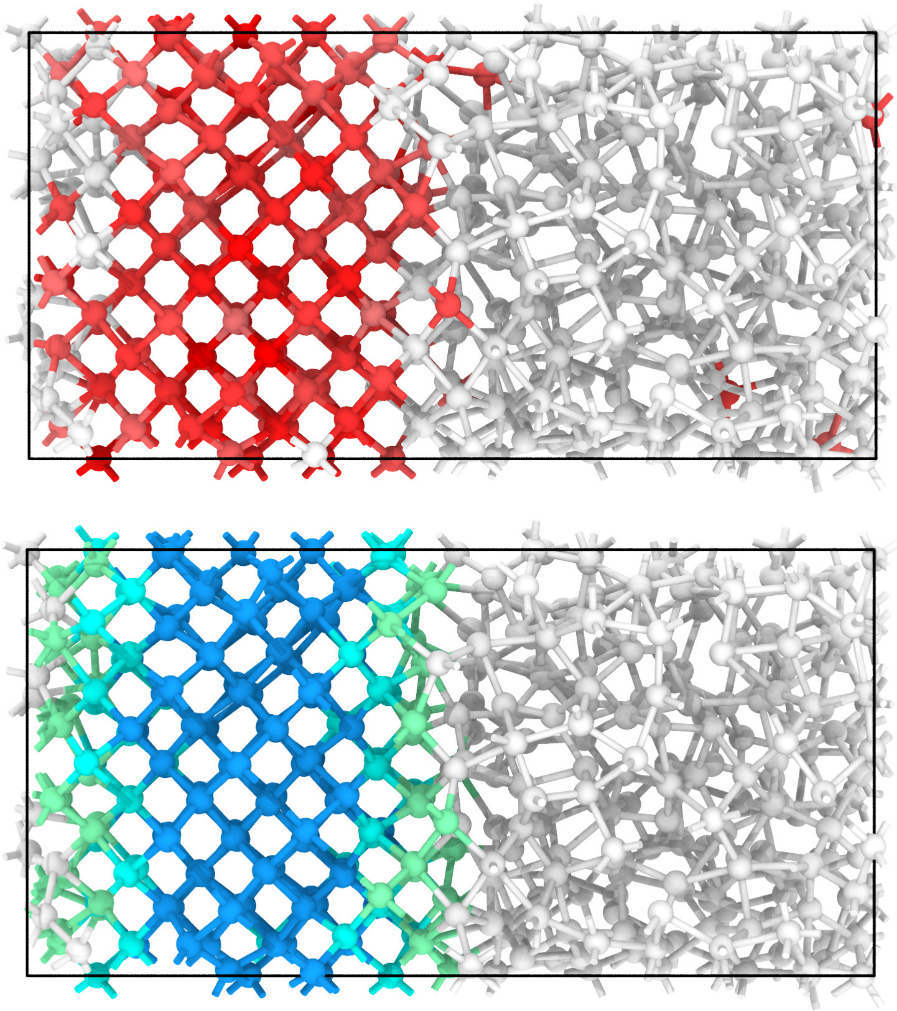

FIG. SI-4. Solid-Liquid coexistence, atoms coloured with: (top) local structure factor based on the first peak, above a threshold of 1.25, and (bottom) extended version of Common Neighbor Analysis for identifying diamond arrangements.

[1] S. Plimpton, P. Crozier, and A. Thompson, Sandia National Laboratories **18**, 43 (2007).

[2] G. Bussi, D. Donadio, and M. Parrinello, J. Chem. Phys. **126**, (2007).

[3] M. Parrinello and A. Rahman, J. Appl. Phys. **521**, 14101 (1981).

[4] G. J. Martyna, D. J. Tobias, and M. L. Klein, J. Chem. Phys. **101**, 4177 (1994).

[5] F. H. Stillinger and T. A. Weber, Phys. Rev. B **31**, 5262 (1985).

[6] G. A. Tribello, M. Bonomi, D. Branduardi, C. Camilloni, and G. Bussi, Comput. Phys. Commun. **185**, 604 (2014).

[7] W. Kohn and L. J. Sham, Phys. Rev. **140**, (1965).

[8] J. Vandevondele, M. Krack, F. Mohamed, M. Parrinello, T. Chassaing, and J. Hutter, Comput. Phys. Commun. **167**, 103 (2005).

[9] J. Hutter, M. Iannuzzi, F. Schiffmann, and J. Vandevondele, Wiley Interdiscip. Rev. Comput. Mol. Sci. **4**, 15 (2014).

[10] M. A. Marques, M. J. Oliveira, and T. Burnus, Comput. Phys. Commun. **183**, 2227 (2012).

[11] S. Goedecker and M. Teter, Phys. Rev. B - Condens. Matter Mater. Phys. **54**, 1703 (1996).

[12] C. Hartwigsen, S. Goedecker, and J. Hutter, Phys. Rev. B - Condens. Matter Mater. Phys. **58**, 3641 (1998).

[13] J. VandeVondele and J. Hutter, J. Chem. Phys. **127**, (2007).

[14] H. Wang, L. Zhang, J. Han, and W. E, Comput. Phys. Commun. **228**, 178 (2018).

[15] J. Behler, Int. J. Quantum Chem. **115**, 1032 (2015).

[16] G. Gutiérrez and B. Johansson, Phys. Rev. B **65**, 104202 (2002).

[17] Z. Lin and L. V. Zhigilei, Phys. Rev. B - Condens. Matter Mater. Phys. **73**, (2006).

[18] A. Stukowski, Model. Simul. Mater. Sci. Eng. **18**, (2010).

[19] H. Niu, P. M. Piaggi, M. Invernizzi, and M. Parrinello, Proc. Natl. Acad. Sci. U. S. A. **115**, 5348 (2018).
